# Supplementary material for: Latent RANSAC
Source: arXiv:1802.07045 ancillary file (2018-06-03)
Supplement: Supplementary file 1 [file supp.pdf]

# Latent RANSAC
# Supplementary Material

Simon Korman
Weizmann Institute of Science, Israel

Roee Litman
General Motors, Israel

## 1. Parameter selection

The parameters of our methods were fixed for all experiments in the main paper and the ones presented here. These values were empirically selected on synthetic data (disjoint from other experiments), in a procedure detailed below

### 1.1. LR tolerance for inliers

We wish to verify that the collision tolerance in the latent space depends linearly on the inlier noise, much like its RANSAC counterpart. This, in turn, allows us to verify that we will not miss true collisions (prevent false negatives) that may fall too far in the latent domain. A synthetic experiment is performed on several randomly generated "ground-truth" models, each with a set noisy inliers. We then pick a minimal subset of inliers, and assess the resulting "hypothesis", specifically the $\ell_\infty$ distance from the ground-truth which is used by the Random-Grids. Figure 1 presents the median and 90 percentile of these measurements for different noise levels, for each of the three model types we present in the paper.

**Embedding ratio for $SE(3)$.** As mentioned in the paper, for both PnP and rigid-3d estimation problems, we parameterize the special Euclidean group $SE(3)$ as a concatenation of two 3-tuples - one for rotation and one for translation. Figure 1 shows values separately for each of the two tuples. We chose a fixed tolerance ratio between rotation and translation for embedding based on the ratio of the incline for median distance (solid lines in Figure 1). The following values were used in all of our experiments: $1.47\frac{rad}{cm}$ for PnP, and $3.6\frac{rad}{cm}$ for rigid 3D.

### 1.2. Latent tolerance vs. RANSAC tolerance

The previous experiment showed that, much like with RANSAC, the LR tolerance grows linearly with the inlier noise. Hence, there exists a ratio between RANSAC tolerance and that of LR. While this could be done using only inliers (in a synthetic setup, as in the previous experiment), we prefer to see the affect of the tolerance on the outliers as well as part of the complete RANSAC estimation pipeline. Figure 2 depicts the performance of LR in terms of run-time and success rate, as a function of the tolerance value. We measure the tolerance w.r.t. the (fixed) value we used for RANSAC tolerance in all our runs. The chosen ratios (LR-threshold divided by RANSAC-threshold) are 8.75 for Homography, 1.75 for PnP and 1.74 for Rigid-3D.

## 2. Hash table implementation details

The hashing scheme presented in Section 2.2 in the paper can result in an integer $\tau_{\mathbf{v}}$ with a very large number of bits (e.g. over 32), which implies prohibitive memory allocation costs. A common workaround in the hashing literature is to map the result into a smaller range of size $2^b$ which can be described by vectors of $b$ bits. This can be done using any off-the-shelf standard hash function. In our case we simply take the original large number modulo a large prime number with $b$ bits. Note that since any such 'range shrinking' hash function is in particular an injective function, it can not eliminate any original collisions. Taking a small number of bits $b$ saves in memory, while potentially introducing false collisions (that are quickly discarded by a constant time test in the latent space). We take the size of the small range to be $10\%$ of $n = 5 \times 10^6$, which is the maximal number of iterations allowed. In such a case, for a well behaved hash function, the expected number of false collisions is a small constant fraction of $n$.

## 3. Additional results

In this section we provide detailed results which extend those presented in the paper (for completeness we recite the summarized results (Tables 1 and 2 from the paper).

For homography estimation (extending Section 3.1 of the paper), we provide here our results on the dataset by Mikolajczyk *et al.* [3], being a golden standard evaluation benchmark for homography estimation. We use all possible ordered pairs of the 'viewpoint' sequences (each including 6 images): 'graffiti-5', 'graffiti-4', 'bark', 'wall' and 'graffiti'.

Note that the estimation benchmark we put together (described in the paper) using the Zurich Buildings data-set

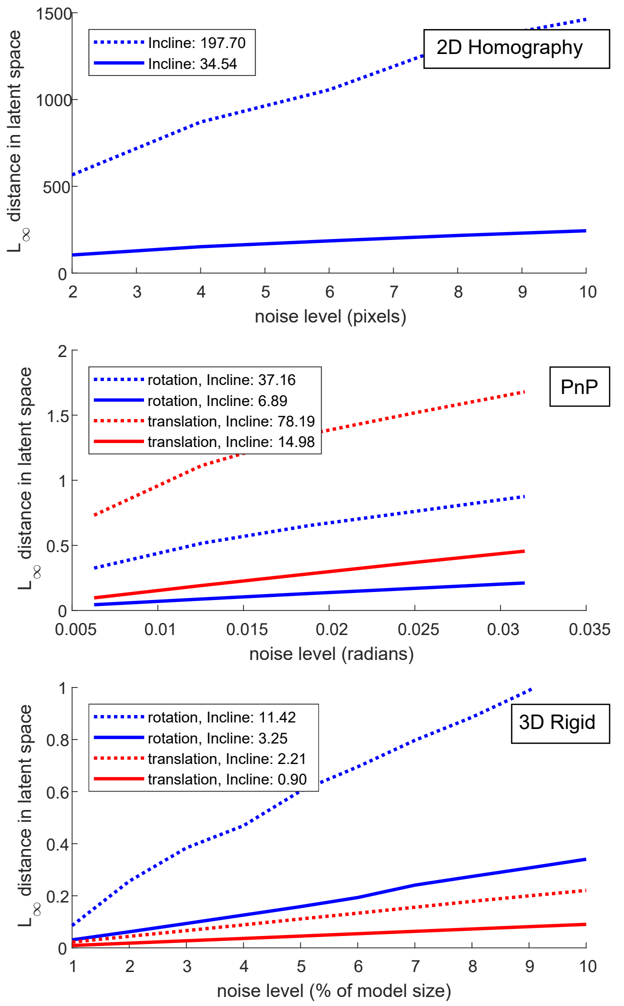


Figure 1. **Embedding $\ell_\infty$ distance for noisy inliers.** For each of the three domains, we show the median (solid) and 90% (dotted) $\ell_\infty$ distance between two inlier hypothesis, as a function of the inlier noise. As can be seen, the embedding distance grows linearly with the noise level, which is a desirable property, observable also in RANSAC tolerance. The resulting incline can be used to select LR tolerance. For PnP and rigid 3D we present the distance for rotation (blue) and translation (red) separately, allowing us to select embedding ratios for the two into the same space.

(ZuBuD) [4] is much larger (1878 vs. 73 pairs) and is much more challenging in terms of inlier rates. See Figure 3 for the cumulative inlier rate distribution in comparison to the other data-sets used in the paper.

For PnP estimation we extend Section 3.2 of the paper by adding a second sequence from the PoseNet data-set, the 'Street' scene that includes 2907 instances. The cumulative inlier rate distribution of Figure 3 shows that it is much more challenging compared to the 'Old Hospital' scene presented in the paper.

For each of the 4 data-sets, we provide summarizing tables in Section 3.1, detailed component invocation and runtime analysis in Section 3.2 and finally - some detailed qualitative examples in Section 3.3.

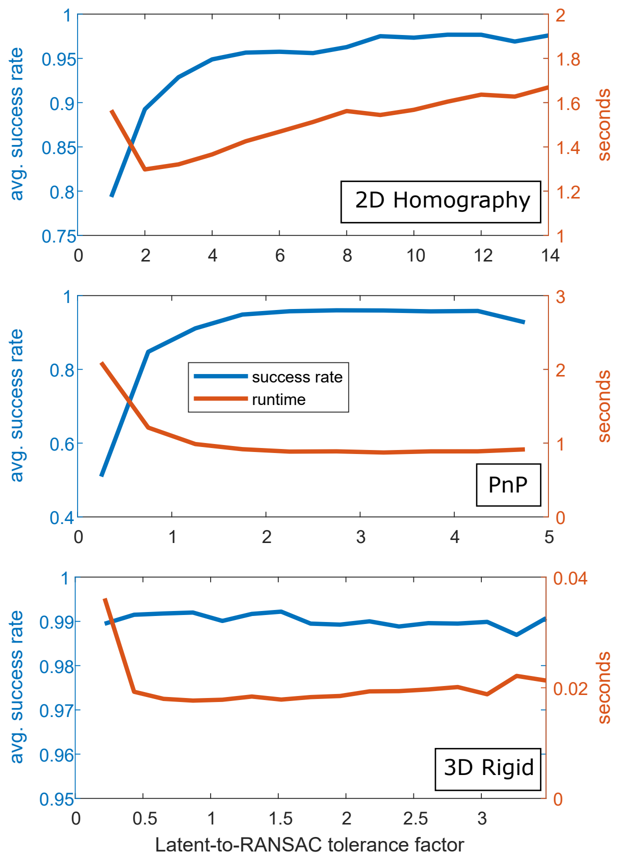


Figure 2. **Robustness of the LR tolerance.** For each of the three domains, we present the ratio between the (fixed) RANSAC tolerance and that of LR. Above a certain value the performance of LR is steady for PnP and rigid 3D, while a slight rise in runtime is evident for 2D homography

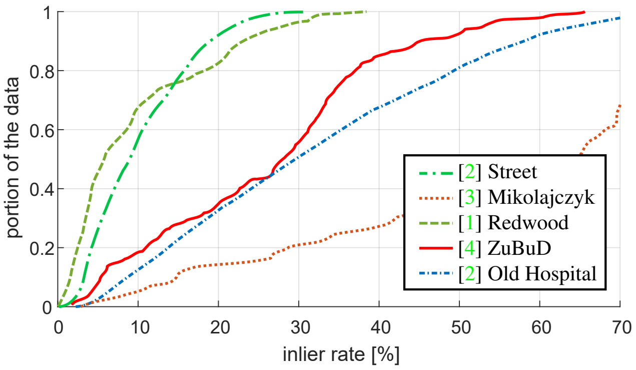


Figure 3. **Inlier rate cumulative distribution** (CDF) of the real data sets we use. The Mikolajczyk data-set [3] added here (compared to Figure 5 of the paper) can be seen to be much less challenging in terms the distribution of inlier rates.

### 3.1. Summarizing tables

The following four tables provide summary results for each of the four tested data-sets, organized by ranges of inlier rates. For each inlier-rate range, we specify the number of instances, provide average and 95th percentile of runtime (in milliseconds), as well as average success rates (which are as a percentage of the optimal inlier rate).

Overall, LR performs in par with the other methods, but excels especially in the more challenging lower inlier rate cases. These data-sets include many such hard examples and hence the impact on the runtime and accuracy measured on the entire data-set can be very significant.

| | | **inlier rate range (in %)** | | | |
|---|---|---|---|---|---|
| **measure** | **method** | 0-10 | 10-20 | 20-40 | 40-100 |
| **runtime** avg. (95%) (millisecs) | RANSAC | 1,490 (6,594) | 35 (97) | 5 (10) | **6 (9)** |
| | SPRT | **1,129** (4,659) | **23 (62)** | **4 (7)** | **6 (9)** |
| | LR | 1,209 **(4,626)** | 32 (85) | 7 (11) | 9 (12) |
| **success** | RANSAC | **93.39%** | 95.53% | 96.28% | 97.33% |
| | SPRT | 88.57% | 95.71% | 96.27% | 97.48% |
| | LR | 93.07% | **95.88%** | **96.55%** | **97.59%** |
| **# of instances** | | 234 | 378 | 655 | 611 |

Table 1. **2D Homography fitting on Zurich Buildings [4].** Best results are shown in bold. See text for further details.

| | | **inlier rate range (in %)** | | | |
|---|---|---|---|---|---|
| **measure** | **method** | 0-10 | 10-20 | 20-40 | 40-100 |
| **runtime** avg. (95%) (millisecs) | RANSAC | 4.2e4 (1.7e5) | 2,336 (5,347) | 190 (471) | 41 (71) |
| | SPRT | 2,760 (1.7e4) | 40 **(71)** | 15 (20) | **12** (16) |
| | LR | **913 (4,403)** | **39** (72) | **14 (18)** | **12 (15)** |
| **success** | RANSAC | **95.54%** | 98.13% | 99.38% | 99.12% |
| | SPRT | 91.94% | **98.23%** | **99.40%** | **99.17%** |
| | LR | 94.73% | 98.14% | 99.39% | 99.11% |
| **# of instances** | | 29 | 27 | 91 | 35 |

Table 2. **PnP fitting on the OldHospital scene from PoseNet [2].** Best results are shown in bold. See text for further details.

| | | **inlier rate range (in %)** | | | |
|---|---|---|---|---|---|
| **measure** | **method** | 0-10 | 10-20 | 20-40 | 40-100 |
| **runtime** avg. (95%) (millisecs) | RANSAC | 3,324 (8,433) | 36 (81) | 6 **(7)** | **14 (22)** |
| | SPRT | 2,395 (4,661) | **21 (46)** | **5 (7)** | **14 (22)** |
| | LR | **2,063 (4,631)** | 28 (60) | 8 (10) | 17 (25) |
| **success** | RANSAC | **91.45%** | 97.85% | 99.11% | **99.41%** |
| | SPRT | 61.86% | 98.02% | 99.30% | **99.41%** |
| | LR | 90.32% | **98.04%** | **99.33%** | 99.40% |
| **# of instances** | | 4 | 7 | 9 | 53 |

Table 3. **Homography fitting on the Viewpoint sequences from the Mikolajczyk data-set [3].** Best results are shown in bold. See text for further details.

### 3.2. Additional empirical runtime analysis

In the right column of Figure 4 we reiterate the runtime breakdown presented in Figure 6 in the paper, for PnP estimation (on the 'Old Hospital' and 'Street' scenes of the

| | | **inlier rate range (in %)** | | |
|---|---|---|---|---|
| **measure** | **method** | 0-4 | 4-6 | 6-100 |
| **runtime** avg. (95%) (millisecs) | RANSAC | 8.6e4 (1.6e5) | 2.9e4 (5.9e4) | 4.2e3 (1.3e4) |
| | SPRT | 2.4e4 (5.1e4) | 1.4e3 (2.7e3) | **1.2e2** (3.7e2) |
| | LR | **2.3e3 (4.2e3)** | **8.8e2 (1.6e3)** | 1.0e2 **(2.9e2)** |
| **success** | RANSAC | **95.37%** | 95.67% | 98.83% |
| | SPRT | 60.69% | **95.87%** | **98.84%** |
| | LR | 89.89% | 90.72% | 97.95% |
| **# of instances** | | 844 | 1037 | 1026 |

Table 4. **PnP fitting on the Street scene from PoseNet [2].** Best results are shown in bold. See text for further details.

PoseNet [2] dataset) and for homography estimation (on Mikolajczyk [3] and ZuBuD [4] data-sets). We also provide two additional views: In the left column, we show the ($\log_{10}$ of the) average number of invocations per module, while in the middle column we show the relative module runtimes (i.e. as a fraction of the total runtime).

The left column (number of activations) emphasizes the fact that in the case of Latent-RANSAC each fitted model is then hashed (hence the equal number of fitting and hashing activations), while few hypotheses need to be verified (following a collision) compared to the other methods (notice the log10 x-scale). Looking at the *relative* time per module (middle column), it is evident that Latent-RANSAC spends only a small fraction of its time on model verification in comparison with the other methods, while it needs to handle hypothesis hashing, which is much less time consuming. Notice also that LR requires a longer initialization time to set up the hash tables.

### 3.3. Qualitative examples

In tables 9, 10, 11 and 12 we collected several representative examples for each of the 'Old Hospital' and 'Street' scenes from the PoseNet dataset [2], the Mikolajczyk [3] and Zurich Buildings (ZuBuD) [4] dataset, respectively. All results are specified in median ± std format, over 10, 2, 100 and 10 iterations per instance, for each of the data-set respectively.

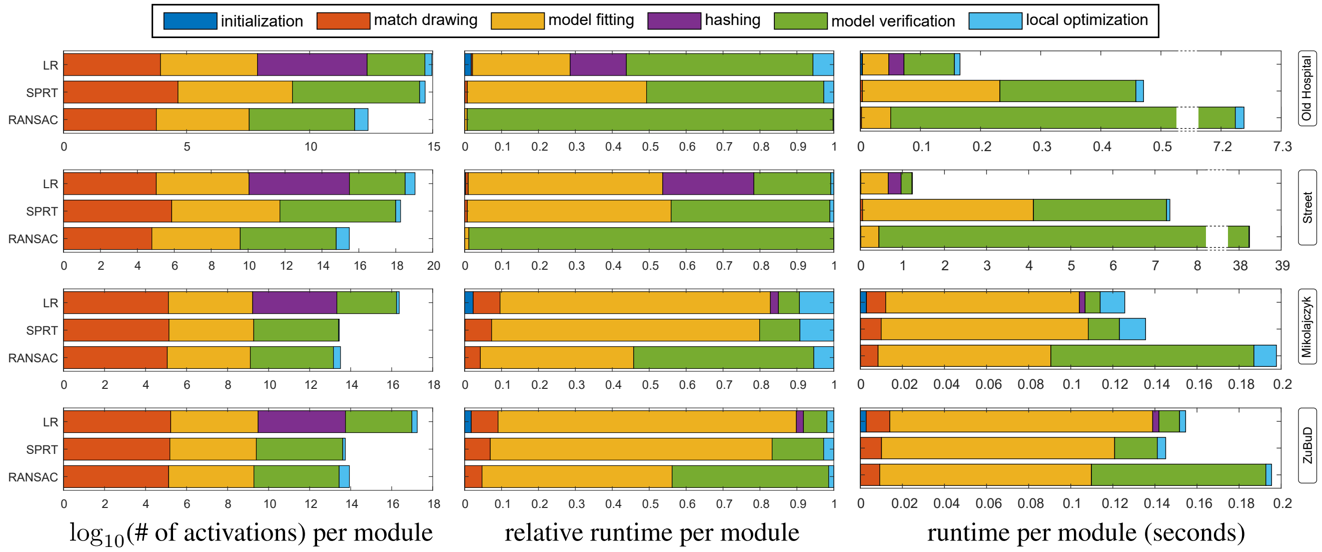


Figure 4. **Details on sub-module invocations and runtimes**: The presented values are averages (per single run) over the entire data. Each row corresponds to a different dataset - The top two rows relate to the 'Old Hospital' and 'Street' scenes from the PoseNet dataset [2], which we use for PnP estimation. The bottom two rows relate to the Mikolajczyk [3] and Zurich Buildings (ZuBuD) [4] dataset, which we use for Homography estimation. Each column gives a different kind of information; **left** $\log_{10}$ of the number of times each module was invoked per single run. **middle**: module runtime as a fraction of total time. **bottom**: average runtime of each module.

| *image pair* | *measure* | USAC | SPRT | LR |
|---|---|---|---|---|
| **Street image 2 frame 535** | inlier rate (%) | 2.5±0.1 | 0.0±0.0 | 2.4±0.2 |
| #matches: 8345 | Sampson err. | 0.8±0.2 | 3.1±0.0 | 0.5±0.0 |
| | #samples | 306037±24889 | 5000000±0 | 467546±30370 |
| 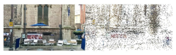 | #fitting | 306037±24889 | 5000000±0 | 467546±30370 |
| | #verification | 783585±64107 | 12812862±1737 | 4767±420 |
| | runtime [sec] | 293.192±30.115 | 41.311±0.848 | 6.020±1.096 |
| **Street image 1 frame 231** | inlier rate (%) | 2.9±0.1 | 0.0±0.0 | 2.8±0.1 |
| #matches: 4797 | Sampson err. | 0.3±0.2 | 3.1±0.0 | 0.4±0.0 |
| | #samples | 187160±10964 | 5000000±0 | 323861±30751 |
| 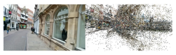 | #fitting | 187160±10964 | 5000000±0 | 323861±30751 |
| | #verification | 483498±28250 | 12911343±3440 | 3623±598 |
| | runtime [sec] | 105.653±9.589 | 41.944±0.746 | 3.647±0.642 |
| **Street image 2 frame 323** | inlier rate (%) | 2.9±0.1 | 0.0±0.0 | 2.8±0.1 |
| #matches: 5796 | Sampson err. | 0.2±0.0 | 3.1±0.0 | 0.4±0.0 |
| | #samples | 195970±19780 | 5000000±0 | 326970±47173 |
| 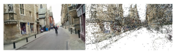 | #fitting | 195970±19780 | 5000000±0 | 326970±47173 |
| | #verification | 508034±51175 | 12969247±1982 | 3918±846 |
| | runtime [sec] | 125.608±15.425 | 41.823±0.331 | 3.929±0.628 |
| **Street image 2 frame 1212** | inlier rate (%) | 3.2±0.1 | 3.2±1.7 | 3.1±0.1 |
| #matches: 7518 | Sampson err. | 0.7±0.0 | 0.4±1.4 | 0.4±0.0 |
| | #samples | 142419±8773 | 4181223±1707519 | 219329±31236 |
| 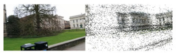 | #fitting | 142419±8773 | 4181223±1707519 | 219329±31236 |
| | #verification | 380804±23487 | 11175766±4563988 | 3136±739 |
| | runtime [sec] | 129.371±9.946 | 38.178±15.573 | 2.951±0.609 |
| **Street image 2 frame 94** | inlier rate (%) | 3.3±0.2 | 3.2±1.7 | 3.1±0.1 |
| #matches: 1747 | Sampson err. | 0.5±0.0 | 0.4±1.4 | 0.4±0.0 |
| | #samples | 129519±21199 | 3492047±1685548 | 244691±37878 |
| 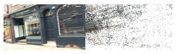 | #fitting | 129519±21199 | 3492047±1685548 | 244691±37878 |
| | #verification | 325452±53201 | 8783411±4240297 | 2018±436 |
| | runtime [sec] | 24.603±3.649 | 27.864±13.291 | 2.171±0.252 |
| **Street image 2 frame 880** | inlier rate (%) | 3.5±0.1 | 3.5±0.1 | 3.4±0.1 |
| #matches: 6683 | Sampson err. | 0.3±0.5 | 0.3±0.2 | 0.7±0.2 |
| | #samples | 108629±5369 | 402561±154146 | 171161±12160 |
| 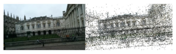 | #fitting | 108629±5369 | 402561±154146 | 171161±12160 |
| | #verification | 303855±14732 | 1126568±431003 | 3618±476 |
| | runtime [sec] | 88.889±7.535 | 3.989±1.257 | 2.519±0.389 |
| **Street image 2 frame 2392** | inlier rate (%) | 3.5±0.2 | 3.5±0.1 | 3.3±0.2 |
| #matches: 2954 | Sampson err. | 0.7±0.1 | 0.4±0.1 | 0.5±0.0 |
| | #samples | 111756±13065 | 300486±91916 | 184796±23830 |
| 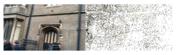 | #fitting | 111756±13065 | 300486±91916 | 184796±23830 |
| | #verification | 286412±33513 | 769610±235189 | 1523±278 |
| | runtime [sec] | 35.420±5.480 | 2.908±0.657 | 1.850±0.378 |
| **Street image 2 frame 628** | inlier rate (%) | 3.8±0.1 | 3.9±0.1 | 3.6±0.2 |
| #matches: 4789 | Sampson err. | 0.8±0.0 | 0.5±0.0 | 0.4±0.0 |
| | #samples | 82497±4777 | 182585±15613 | 135563±21892 |
| 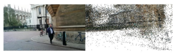 | #fitting | 82497±4777 | 182585±15613 | 135563±21892 |
| | #verification | 217991±12614 | 483672±41081 | 1520±361 |
| | runtime [sec] | 45.438±5.229 | 1.987±0.148 | 1.522±0.258 |

Table 5. **STREET SUBSET on pnp dataset.**

| *image pair* | *measure* | USAC | SPRT | LR |
|---|---|---|---|---|
| **Street image 2 frame 11** | inlier rate (%) | 3.4±0.3 | 3.5±1.2 | 2.9±0.2 |
| #matches: 3067 | Sampson err. | 0.7±0.2 | 0.4±0.9 | 0.5±0.1 |
| | #samples | 127107±24168 | 1554596±1303455 | 272706±45448 |
| 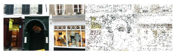 | #fitting | 127107±24168 | 1554596±1303455 | 272706±45448 |
| | #verification | 320979±60997 | 3919077±3288015 | 2204±556 |
| | runtime [sec] | 39.850±7.647 | 12.853±10.419 | 2.448±0.541 |
| **Street image 2 frame 1666** | inlier rate (%) | 4.2±0.0 | 4.2±0.0 | 4.1±0.3 |
| #matches: 7010 | Sampson err. | 2.3±0.1 | 2.2±0.1 | 1.5±0.5 |
| | #samples | 65015±492 | 135570±9172 | 93418±30836 |
| 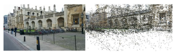 | #fitting | 65015±492 | 135570±9172 | 93418±30836 |
| | #verification | 172052±1366 | 359514±24156 | 846±465 |
| | runtime [sec] | 54.031±4.484 | 1.278±0.106 | 1.161±0.467 |
| **Street image 2 frame 1125** | inlier rate (%) | 4.0±0.2 | 4.1±0.2 | 3.3±0.2 |
| #matches: 5643 | Sampson err. | 2.8±1.3 | 0.5±0.8 | 0.4±0.2 |
| | #samples | 81631±10960 | 204675±41212 | 190577±23379 |
| 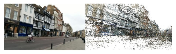 | #fitting | 81631±10960 | 204675±41212 | 190577±23379 |
| | #verification | 212994±28781 | 533496±107449 | 2597±467 |
| | runtime [sec] | 51.271±6.048 | 2.254±0.375 | 2.158±0.423 |
| **Street image 2 frame 240** | inlier rate (%) | 4.2±0.0 | 4.2±0.0 | 4.2±0.0 |
| #matches: 5883 | Sampson err. | 2.2±0.0 | 2.8±0.0 | 2.5±0.0 |
| | #samples | 60704±495 | 126088±9888 | 84986±533 |
| 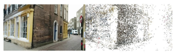 | #fitting | 60704±495 | 126088±9888 | 84986±533 |
| | #verification | 158126±1164 | 327457±25629 | 518±19 |
| | runtime [sec] | 41.052±1.998 | 1.164±0.083 | 0.875±0.097 |
| **Street image 2 frame 1680** | inlier rate (%) | 4.5±0.0 | 4.5±0.0 | 4.5±0.0 |
| #matches: 7313 | Sampson err. | 0.9±0.0 | 0.7±0.0 | 0.4±0.0 |
| | #samples | 52444±573 | 103368±8042 | 73422±733 |
| 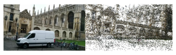 | #fitting | 52444±573 | 103368±8042 | 73422±733 |
| | #verification | 139939±1494 | 275663±21392 | 510±20 |
| | runtime [sec] | 46.688±4.115 | 0.934±0.092 | 0.862±0.083 |
| **Street image 2 frame 638** | inlier rate (%) | 4.3±0.1 | 4.3±0.1 | 3.8±0.4 |
| #matches: 2435 | Sampson err. | 0.8±0.1 | 0.5±0.0 | 0.5±0.0 |
| | #samples | 58203±5124 | 133526±12030 | 147731±50759 |
| 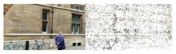 | #fitting | 58203±5124 | 133526±12030 | 147731±50759 |
| | #verification | 147051±13042 | 337307±30361 | 889±429 |
| | runtime [sec] | 14.777±1.767 | 1.172±0.113 | 1.058±0.546 |
| **Street image 2 frame 2258** | inlier rate (%) | 4.7±0.0 | 4.7±0.0 | 4.7±0.0 |
| #matches: 8043 | Sampson err. | 1.6±0.0 | 1.5±0.0 | 1.5±0.0 |
| | #samples | 45057±152 | 86100±6798 | 63080±6191 |
| 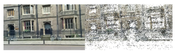 | #fitting | 45057±152 | 86100±6798 | 63080±6191 |
| | #verification | 114502±512 | 218806±17224 | 366±55 |
| | runtime [sec] | 41.804±2.848 | 0.776±0.057 | 0.670±0.090 |
| **Street image 2 frame 1390** | inlier rate (%) | 4.6±0.1 | 4.6±0.1 | 4.4±0.2 |
| #matches: 3910 | Sampson err. | 0.3±0.0 | 0.4±0.1 | 0.4±0.0 |
| | #samples | 46777±3889 | 90591±9725 | 79851±10445 |
| 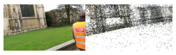 | #fitting | 46777±3889 | 90591±9725 | 79851±10445 |
| | #verification | 125606±10455 | 242952±26149 | 1082±218 |
| | runtime [sec] | 20.304±2.659 | 1.071±0.115 | 0.790±0.182 |

Table 6. **STREET SUBSET on pnp dataset.**

| *image pair* | *measure* | USAC | SPRT | LR |
|---|---|---|---|---|
| **Street image 2 frame 604** | inlier rate (%) | 4.8±0.1 | 4.9±0.1 | 4.8±0.1 |
| #matches: 3757 | Sampson err. | 2.4±0.0 | 2.7±0.0 | 2.8±0.0 |
| | #samples | 41841±1644 | 74948±3271 | 62711±32819 |
| 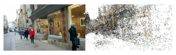 | #fitting | 41841±1644 | 74948±3271 | 62711±32819 |
| | #verification | 109549±4361 | 196167±8754 | 355±289 |
| | runtime [sec] | 17.572±1.286 | 0.638±0.027 | 0.677±0.363 |
| **Street image 2 frame 258** | inlier rate (%) | 4.7±0.3 | 4.7±0.2 | 4.0±0.3 |
| #matches: 2127 | Sampson err. | 0.6±0.0 | 0.3±0.0 | 0.4±0.0 |
| | #samples | 47020±9372 | 79779±19126 | 102716±20137 |
| 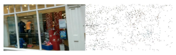 | #fitting | 47020±9372 | 79779±19126 | 102716±20137 |
| | #verification | 121312±24211 | 205828±49464 | 751±216 |
| | runtime [sec] | 10.804±2.424 | 0.707±0.175 | 0.941±0.289 |
| **Street image 1 frame 155** | inlier rate (%) | 4.8±0.1 | 4.8±0.2 | 4.7±0.2 |
| #matches: 8064 | Sampson err. | 0.8±0.3 | 0.3±0.3 | 0.4±0.3 |
| | #samples | 42093±3754 | 81062±8369 | 63576±8158 |
| 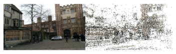 | #fitting | 42093±3754 | 81062±8369 | 63576±8158 |
| | #verification | 109315±9719 | 210591±21876 | 414±86 |
| | runtime [sec] | 40.997±4.340 | 0.703±0.085 | 0.652±0.112 |
| **Street image 2 frame 2439** | inlier rate (%) | 5.3±0.0 | 5.3±0.0 | 5.3±0.0 |
| #matches: 6287 | Sampson err. | 2.0±0.0 | 2.0±0.1 | 2.0±0.0 |
| | #samples | 30698±217 | 52672±3010 | 43365±9916 |
| 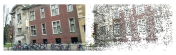 | #fitting | 30698±217 | 52672±3010 | 43365±9916 |
| | #verification | 75692±518 | 130108±7439 | 143±33 |
| | runtime [sec] | 21.293±1.446 | 0.440±0.020 | 0.407±0.122 |
| **Street image 2 frame 1908** | inlier rate (%) | 6.0±0.0 | 6.0±0.0 | 6.0±0.0 |
| #matches: 5187 | Sampson err. | 2.7±0.0 | 2.7±0.0 | 2.5±0.0 |
| | #samples | 21147±231 | 34980±1817 | 29465±2816 |
| 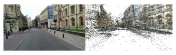 | #fitting | 21147±231 | 34980±1817 | 29465±2816 |
| | #verification | 55818±700 | 92217±4813 | 156±37 |
| | runtime [sec] | 12.741±1.143 | 0.305±0.014 | 0.318±0.049 |
| **Street image 2 frame 1236** | inlier rate (%) | 6.9±0.0 | 6.9±0.0 | 6.9±0.0 |
| #matches: 4241 | Sampson err. | 2.3±0.0 | 1.6±0.0 | 0.0±0.0 |
| | #samples | 14243±169 | 22629±1736 | 20253±570 |
| 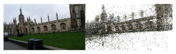 | #fitting | 14243±169 | 22629±1736 | 20253±570 |
| | #verification | 39898±453 | 63106±4902 | 161±16 |
| | runtime [sec] | 7.227±0.598 | 0.200±0.010 | 0.229±0.032 |
| **Street image 2 frame 1179** | inlier rate (%) | 8.4±0.1 | 8.4±0.1 | 8.4±0.1 |
| #matches: 5501 | Sampson err. | 0.4±0.0 | 0.2±0.0 | 1.4±0.0 |
| | #samples | 7718±216 | 11311±599 | 10841±548 |
| 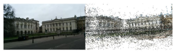 | #fitting | 7718±216 | 11311±599 | 10841±548 |
| | #verification | 21428±636 | 31689±1670 | 79±11 |
| | runtime [sec] | 5.225±0.389 | 0.112±0.013 | 0.126±0.019 |
| **Street image 2 frame 1532** | inlier rate (%) | 8.6±0.1 | 8.6±0.0 | 8.6±0.0 |
| #matches: 6711 | Sampson err. | 2.2±0.1 | 1.9±0.0 | 0.8±0.0 |
| | #samples | 7241±128 | 10261±874 | 10351±1907 |
| 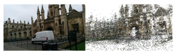 | #fitting | 7241±128 | 10261±874 | 10351±1907 |
| | #verification | 19629±436 | 27720±2378 | 30±10 |
| | runtime [sec] | 6.057±0.340 | 0.090±0.003 | 0.115±0.024 |

Table 7. **STREET SUBSET on pnp dataset.**

| *image pair* | *measure* | USAC | SPRT | LR |
|---|---|---|---|---|
| **Street image 2 frame 2145** | inlier rate (%) | 9.1±0.2 | 9.1±0.1 | 9.1±0.1 |
| #matches: 5395 | Sampson err. | 0.3±0.0 | 0.3±0.0 | 0.3±0.0 |
| | #samples | 6179±304 | 8892±424 | 8651±304 |
| 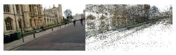 | #fitting | 6179±304 | 8892±424 | 8651±304 |
| | #verification | 16636±863 | 23917±1179 | 33±6 |
| | runtime [sec] | 3.920±0.275 | 0.078±0.006 | 0.096±0.010 |
| **Street image 2 frame 1153** | inlier rate (%) | 12.2±0.0 | 12.2±0.0 | 12.2±0.0 |
| #matches: 4088 | Sampson err. | 1.1±0.0 | 1.7±0.0 | 2.8±0.0 |
| | #samples | 2559±11 | 3346±267 | 3605±9 |
| 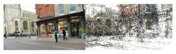 | #fitting | 2559±11 | 3346±267 | 3605±9 |
| | #verification | 6758±58 | 8758±684 | 11±3 |
| | runtime [sec] | 1.223±0.113 | 0.028±0.002 | 0.037±0.006 |
| **Street image 2 frame 1806** | inlier rate (%) | 13.5±0.0 | 13.5±0.0 | 13.5±0.0 |
| #matches: 8868 | Sampson err. | 1.6±0.0 | 1.8±0.0 | 2.1±0.0 |
| | #samples | 1884±6 | 2391±109 | 2632±240 |
| 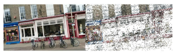 | #fitting | 1884±6 | 2391±109 | 2632±240 |
| | #verification | 4588±34 | 5887±321 | 8±5 |
| | runtime [sec] | 1.888±0.116 | 0.031±0.003 | 0.038±0.007 |
| **Street image 2 frame 972** | inlier rate (%) | 15.1±0.0 | 15.1±0.0 | 15.1±0.0 |
| #matches: 4606 | Sampson err. | 1.1±0.0 | 2.2±0.0 | 2.5±0.0 |
| | #samples | 1338±11 | 1510±133 | 1874±14 |
| 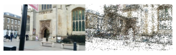 | #fitting | 1338±11 | 1510±133 | 1874±14 |
| | #verification | 3467±68 | 3949±313 | 5±2 |
| | runtime [sec] | 0.719±0.054 | 0.021±0.003 | 0.028±0.003 |
| **Street image 1 frame 16** | inlier rate (%) | 16.4±0.0 | 16.4±0.0 | 16.4±0.0 |
| #matches: 4742 | Sampson err. | 1.7±0.0 | 2.4±0.0 | 2.1±0.0 |
| | #samples | 1036±3 | 1184±102 | 1454±19 |
| 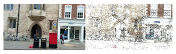 | #fitting | 1036±3 | 1184±102 | 1454±19 |
| | #verification | 2554±42 | 2975±226 | 6±3 |
| | runtime [sec] | 0.533±0.050 | 0.016±0.002 | 0.022±0.003 |
| **Street image 2 frame 2022** | inlier rate (%) | 18.1±0.1 | 18.1±0.2 | 18.1±0.1 |
| #matches: 5155 | Sampson err. | 0.9±0.0 | 0.9±0.0 | 1.1±0.0 |
| | #samples | 780±10 | 951±47 | 1088±28 |
| 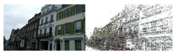 | #fitting | 780±10 | 951±47 | 1088±28 |
| | #verification | 1999±38 | 2460±133 | 7±3 |
| | runtime [sec] | 0.461±0.033 | 0.016±0.003 | 0.021±0.005 |

Table 8. **STREET SUBSET on pnp dataset.**

| *image pair* | *measure* | USAC | SPRT | LR |
|---|---|---|---|---|
| **OldHospital seq 8 frame 12** | inlier rate (%) | 2.9±0.1 | 0.0±0.0 | 2.9±0.1 |
| #matches: 9917 | Sampson err. | 0.5±0.1 | 3.1±0.0 | 0.4±0.1 |
| 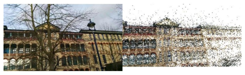 | #samples | 190937±11435 | 5000000±0 | 256422±34273 |
| | #fitting | 190937±11435 | 5000000±0 | 256422±34273 |
| | #verification | 625489±37275 | 16368915±1753 | 10876±2160 |
| | runtime [sec] | 270.965±20.834 | 49.785±2.298 | 6.854±1.331 |
| **OldHospital seq 8 frame 11** | inlier rate (%) | 3.4±0.1 | 3.3±1.1 | 3.3±0.1 |
| #matches: 9141 | Sampson err. | 0.2±0.0 | 0.2±0.9 | 0.2±0.0 |
| 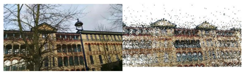 | #samples | 121599±10152 | 1474533±1367665 | 185116±25802 |
| | #fitting | 121599±10152 | 1474533±1367665 | 185116±25802 |
| | #verification | 396913±33382 | 4816358±4466653 | 6797±1386 |
| | runtime [sec] | 159.486±12.493 | 14.436±13.681 | 4.218±0.800 |
| **OldHospital seq 4 frame 13** | inlier rate (%) | 3.9±0.1 | 3.9±0.1 | 3.9±0.2 |
| #matches: 6453 | Sampson err. | 0.4±0.1 | 0.4±0.0 | 0.4±0.1 |
| 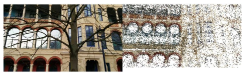 | #samples | 79639±5514 | 198060±53450 | 112847±20268 |
| | #fitting | 79639±5514 | 198060±53450 | 112847±20268 |
| | #verification | 260535±17996 | 647721±174581 | 3446±914 |
| | runtime [sec] | 71.379±6.032 | 2.139±0.606 | 1.851±0.448 |
| **OldHospital seq 4 frame 14** | inlier rate (%) | 4.0±0.2 | 3.9±0.1 | 3.9±0.2 |
| #matches: 6844 | Sampson err. | 0.5±0.0 | 0.5±0.0 | 0.5±0.0 |
| 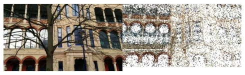 | #samples | 78912±11047 | 190539±42492 | 117709±31943 |
| | #fitting | 78912±11047 | 190539±42492 | 117709±31943 |
| | #verification | 258933±36148 | 624737±139455 | 3606±1639 |
| | runtime [sec] | 74.721±11.198 | 2.147±0.422 | 1.989±0.749 |
| **OldHospital seq 4 frame 16** | inlier rate (%) | 5.5±0.1 | 5.5±0.1 | 5.5±0.1 |
| #matches: 6915 | Sampson err. | 0.6±0.0 | 0.6±0.0 | 0.6±0.0 |
| 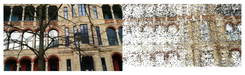 | #samples | 28518±1020 | 49230±3542 | 39766±1828 |
| | #fitting | 28518±1020 | 49230±3542 | 39766±1828 |
| | #verification | 93563±3341 | 161974±11598 | 664±69 |
| | runtime [sec] | 28.043±1.073 | 0.523±0.048 | 0.499±0.036 |
| **OldHospital seq 8 frame 7** | inlier rate (%) | 9.9±0.1 | 9.9±0.1 | 10.0±0.1 |
| #matches: 8608 | Sampson err. | 0.2±0.0 | 0.2±0.0 | 0.2±0.0 |
| 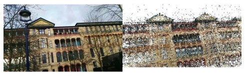 | #samples | 4729±106 | 6479±544 | 6552±110 |
| | #fitting | 4729±106 | 6479±544 | 6552±110 |
| | #verification | 15476±332 | 21121±1802 | 35±6 |
| | runtime [sec] | 5.785±0.229 | 0.078±0.006 | 0.077±0.007 |
| **OldHospital seq 4 frame 46** | inlier rate (%) | 18.7±0.2 | 18.7±0.2 | 18.7±0.0 |
| #matches: 8240 | Sampson err. | 0.4±0.0 | 0.4±0.0 | 0.4±0.0 |
| 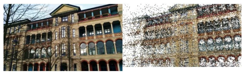 | #samples | 703±24 | 850±71 | 983±81 |
| | #fitting | 703±24 | 850±71 | 983±81 |
| | #verification | 2330±80 | 2825±253 | 6±3 |
| | runtime [sec] | 0.869±0.041 | 0.025±0.005 | 0.024±0.006 |
| **OldHospital seq 8 frame 99** | inlier rate (%) | 67.1±0.0 | 67.1±0.1 | 67.1±0.1 |
| #matches: 5182 | Sampson err. | 0.1±0.0 | 0.1±0.0 | 0.1±0.0 |
| 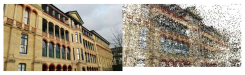 | #samples | 13±0 | 14±1 | 19±3 |
| | #fitting | 13±0 | 14±1 | 19±3 |
| | #verification | 43±3 | 47±4 | 4±2 |
| | runtime [sec] | 0.018±0.004 | 0.011±0.005 | 0.011±0.002 |

Table 9. **Homography estimation on OldHospital scene from PoseNet [2].**

| *image pair* | *measure* | USAC | SPRT | LR |
|---|---|---|---|---|
| **Street image 1 frame 116** | inlier rate (%) | 2.3±0.0 | 0.0±0.0 | 2.2±0.2 |
| #matches: 9685 | Sampson err. | 0.6±0.2 | 3.1±0.0 | 0.6±0.1 |
| | #samples | 401039±11679 | 5000000±0 | 496675±672 |
| 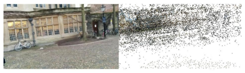 | #fitting | 401039±11679 | 5000000±0 | 496675±672 |
| | #verification | 1009308±28697 | 12573043±6628 | 4885±291 |
| | runtime [sec] | 489.618±12.470 | 50.370±9.862 | 6.918±0.305 |
| **Street image 1 frame 114** | inlier rate (%) | 2.3±0.0 | 0.0±0.0 | 2.1±0.0 |
| #matches: 10316 | Sampson err. | 0.7±0.0 | 3.1±0.0 | 0.5±0.1 |
| | #samples | 382183±10283 | 5000000±0 | 496384±467 |
| 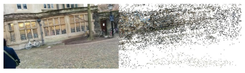 | #fitting | 382183±10283 | 5000000±0 | 496384±467 |
| | #verification | 962421±27524 | 12592970±20 | 4808±65 |
| | runtime [sec] | 498.683±16.713 | 56.789±1.455 | 7.193±0.122 |
| **Street image 2 frame 627** | inlier rate (%) | 3.5±0.1 | 3.5±0.0 | 3.3±0.1 |
| #matches: 5358 | Sampson err. | 0.3±0.0 | 0.3±0.0 | 0.6±0.0 |
| | #samples | 107958±13405 | 262518±28080 | 202990±11599 |
| 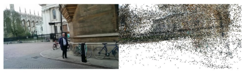 | #fitting | 107958±13405 | 262518±28080 | 202990±11599 |
| | #verification | 278493±35150 | 675917±72078 | 1826±162 |
| | runtime [sec] | 71.865±9.081 | 3.371±0.401 | 2.392±0.140 |
| **Street image 2 frame 2154** | inlier rate (%) | 3.8±0.0 | 3.8±0.0 | 3.8±0.0 |
| #matches: 4313 | Sampson err. | 1.2±0.0 | 2.4±0.0 | 2.3±0.0 |
| | #samples | 86845±0 | 208184±54279 | 120471±1573 |
| 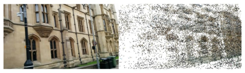 | #fitting | 86845±0 | 208184±54279 | 120471±1573 |
| | #verification | 225467±394 | 541280±141451 | 793±16 |
| | runtime [sec] | 40.972±7.438 | 2.504±0.475 | 1.289±0.055 |
| **Street image 2 frame 2061** | inlier rate (%) | 4.7±0.0 | 4.7±0.0 | 4.7±0.0 |
| #matches: 4423 | Sampson err. | 2.5±0.0 | 0.9±0.0 | 0.9±0.0 |
| | #samples | 45886±473 | 89092±3214 | 63312±651 |
| 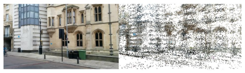 | #fitting | 45886±473 | 89092±3214 | 63312±651 |
| | #verification | 118623±1136 | 230151±7868 | 292±8 |
| | runtime [sec] | 24.092±2.474 | 0.894±0.128 | 0.634±0.043 |
| **Street image 2 frame 2138** | inlier rate (%) | 6.9±0.0 | 6.9±0.0 | 6.9±0.0 |
| #matches: 5056 | Sampson err. | 1.1±0.0 | 2.3±0.0 | 2.3±0.0 |
| | #samples | 13993±170 | 22306±297 | 19423±235 |
| 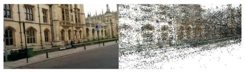 | #fitting | 13993±170 | 22306±297 | 19423±235 |
| | #verification | 37579±440 | 59905±802 | 103±4 |
| | runtime [sec] | 8.137±1.451 | 0.226±0.061 | 0.210±0.027 |
| **Street image 2 frame 1584** | inlier rate (%) | 15.7±0.0 | 15.7±0.0 | 15.7±0.0 |
| #matches: 5859 | Sampson err. | 0.6±0.0 | 2.3±0.0 | 2.1±0.0 |
| | #samples | 1197±3 | 1508±3 | 1671±4 |
| 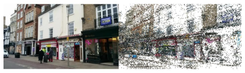 | #fitting | 1197±3 | 1508±3 | 1671±4 |
| | #verification | 2973±26 | 3723±58 | 5±3 |
| | runtime [sec] | 0.776±0.121 | 0.023±0.004 | 0.025±0.007 |
| **Street image 2 frame 2116** | inlier rate (%) | 32.3±0.1 | 32.4±0.1 | 32.4±0.1 |
| #matches: 4381 | Sampson err. | 0.4±0.0 | 2.8±0.0 | 2.7±0.0 |
| | #samples | 144±14 | 145±5 | 188±1 |
| 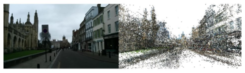 | #fitting | 144±14 | 145±5 | 188±1 |
| | #verification | 405±30 | 393±24 | 5±2 |
| | runtime [sec] | 0.096±0.023 | 0.015±0.004 | 0.018±0.005 |

Table 10. **PnP estimation on Street scene from PoseNet [2].**

| *image pair* | *measure* | USAC | SPRT | LR |
|---|---|---|---|---|
| **graffiti viewpoint views 2 6** | inlier rate (%) | 2.3±0.5 | 0.0±0.0 | 2.0±0.5 |
| #matches: 662 | Sampson err. | 15.0±313.8 | 1056.0±0.0 | 32.1±298.7 |
| 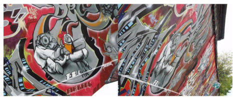 | #samples | 5000006±10 | 5000006±12 | 5000007±7 |
| | #fitting | 488523±653 | 488566±621 | 488503±771 |
| | #verification | 488523±653 | 488566±621 | 38333±530 |
| | runtime [sec] | 8.131±0.409 | 4.372±0.166 | 4.298±0.157 |
| **graffiti viewpoint views 1 5** | inlier rate (%) | 3.9±0.3 | 3.8±1.9 | 3.9±0.2 |
| #matches: 586 | Sampson err. | 7.0±10.1 | 7.6±523.4 | 7.0±7.4 |
| 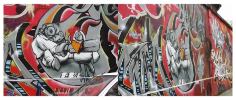 | #samples | 2529197±607021 | 4833036±566999 | 3540872±482973 |
| | #fitting | 247761±59429 | 473514±55468 | 346584±47182 |
| | #verification | 247761±59429 | 473514±55468 | 17316±3438 |
| | runtime [sec] | 4.053±0.922 | 4.234±0.468 | 2.924±0.440 |
| **graffiti 5 viewpoint views 2 6** | inlier rate (%) | 6.7±0.2 | 6.7±0.3 | 6.7±0.3 |
| #matches: 641 | Sampson err. | 3.4±0.9 | 3.4±1.1 | 3.4±2.1 |
| 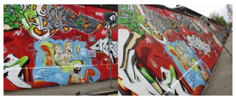 | #samples | 260050±105907 | 293066±121956 | 364065±146559 |
| | #fitting | 25276±10239 | 28427±11742 | 35331±14200 |
| | #verification | 25276±10239 | 28427±11742 | 843±670 |
| | runtime [sec] | 0.420±0.168 | 0.259±0.105 | 0.297±0.125 |
| **wall viewpoint views 1 6** | inlier rate (%) | 8.0±0.2 | 8.0±0.0 | 8.0±0.0 |
| #matches: 722 | Sampson err. | 3.1±0.7 | 3.1±0.1 | 3.3±0.2 |
| 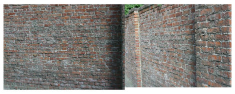 | #samples | 121882±15614 | 131513±5968 | 170633±3328 |
| | #fitting | 12186±1568 | 13108±624 | 17020±366 |
| | #verification | 12186±1568 | 13108±624 | 474±31 |
| | runtime [sec] | 0.213±0.032 | 0.117±0.009 | 0.144±0.009 |
| **graffiti viewpoint views 2 5** | inlier rate (%) | 10.3±0.3 | 10.3±0.2 | 10.3±0.2 |
| #matches: 688 | Sampson err. | 2.2±1.3 | 2.2±0.6 | 2.2±0.7 |
| 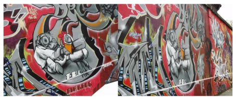 | #samples | 43873±6035 | 45345±3377 | 61412±4514 |
| | #fitting | 4590±634 | 4716±357 | 6365±467 |
| | #verification | 4590±634 | 4716±357 | 81±14 |
| | runtime [sec] | 0.079±0.012 | 0.044±0.004 | 0.056±0.005 |
| **graffiti 5 viewpoint views 3 6** | inlier rate (%) | 10.9±0.2 | 10.9±0.1 | 10.9±0.1 |
| #matches: 724 | Sampson err. | 3.4±0.5 | 3.4±0.4 | 3.4±0.5 |
| 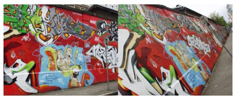 | #samples | 34802±4220 | 35550±1224 | 48720±1671 |
| | #fitting | 3867±487 | 3977±157 | 5410±189 |
| | #verification | 3867±487 | 3977±157 | 50±8 |
| | runtime [sec] | 0.067±0.009 | 0.036±0.003 | 0.047±0.004 |
| **bark Z R views 1 6** | inlier rate (%) | 14.6±0.0 | 14.6±0.0 | 14.6±0.0 |
| #matches: 726 | Sampson err. | 7.0±0.2 | 7.0±0.2 | 7.0±0.2 |
| 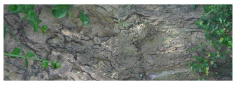 | #samples | 10647±164 | 11291±1041 | 14903±99 |
| | #fitting | 999±31 | 1055±102 | 1391±44 |
| | #verification | 999±31 | 1055±102 | 11±3 |
| | runtime [sec] | 0.019±0.002 | 0.011±0.001 | 0.016±0.001 |
| **graffiti 4 viewpoint views 1 4** | inlier rate (%) | 59.6±0.0 | 59.6±0.0 | 59.6±0.0 |
| #matches: 1117 | Sampson err. | 0.8±0.5 | 0.8±0.6 | 0.8±0.5 |
| 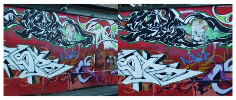 | #samples | 36±2 | 38±3 | 50±8 |
| | #fitting | 12±3 | 13±3 | 18±4 |
| | #verification | 12±3 | 13±3 | 3±2 |
| | runtime [sec] | 0.009±0.003 | 0.010±0.003 | 0.012±0.002 |

Table 11. **Homography estimation on the Viewpoint sequences of Mikolajczyk data-set [3].**

| *image pair* | *measure* | USAC | SPRT | LR |
|---|---|---|---|---|
| **object 155 views 1 3** | inlier rate (%) | 2.0±0.1 | 0.0±0.0 | 2.0±0.2 |
| #matches: 537 | Sampson err. | 537.0±371.6 | 1056.0±0.0 | 141.9±95.9 |
| | #samples | 5000012±6 | 5000007±10 | 5000005±6 |
| 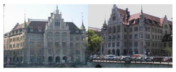 | #fitting | 485267±605 | 485723±696 | 485388±653 |
| | #verification | 485267±605 | 485723±696 | 53017±584 |
| | runtime [sec] | 7.668±0.719 | 4.027±0.332 | 4.198±0.304 |
| **object 116 views 4 5** | inlier rate (%) | 3.1±0.3 | 0.0±0.0 | 3.1±0.4 |
| #matches: 588 | Sampson err. | 16.8±18.3 | 1056.0±0.0 | 19.5±19.6 |
| | #samples | 5000002±99271 | 5000003±5 | 5000009±26 |
| 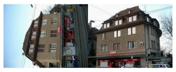 | #fitting | 710936±13857 | 711802±850 | 711487±541 |
| | #verification | 710936±13857 | 711802±850 | 69490±379 |
| | runtime [sec] | 10.731±1.330 | 5.743±0.417 | 6.045±0.454 |
| **object 24 views 1 5** | inlier rate (%) | 4.2±0.3 | 4.5±0.3 | 4.4±0.4 |
| #matches: 516 | Sampson err. | 54.7±108.9 | 35.2±23.8 | 48.7±84.7 |
| | #samples | 2436982±766168 | 2775656±1308085 | 3088939±1194400 |
| 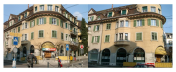 | #fitting | 257719±81008 | 293699±138493 | 326644±126262 |
| | #verification | 257719±81008 | 293699±138493 | 26538±13660 |
| | runtime [sec] | 3.649±1.337 | 2.425±1.303 | 2.798±1.159 |
| **object 109 views 2 5** | inlier rate (%) | 5.0±0.2 | 5.0±0.2 | 5.0±0.1 |
| #matches: 523 | Sampson err. | 65.1±31.0 | 53.0±23.4 | 26.2±28.6 |
| | #samples | 972392±150149 | 1256870±308441 | 1329033±412427 |
| 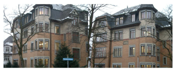 | #fitting | 104526±15924 | 134885±32910 | 142500±44333 |
| | #verification | 104526±15924 | 134885±32910 | 8988±4384 |
| | runtime [sec] | 1.555±0.376 | 1.181±0.301 | 1.176±0.450 |
| **object 122 views 4 5** | inlier rate (%) | 7.6±0.2 | 7.7±0.4 | 7.7±0.3 |
| #matches: 442 | Sampson err. | 47.0±23.2 | 47.4±24.6 | 43.1±25.5 |
| | #samples | 181624±24310 | 202088±28949 | 218094±34407 |
| 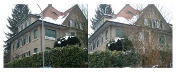 | #fitting | 28236±3788 | 31074±4427 | 33746±5316 |
| | #verification | 28236±3788 | 31074±4427 | 3176±698 |
| | runtime [sec] | 0.365±0.057 | 0.253±0.058 | 0.272±0.054 |
| **object 116 views 2 5** | inlier rate (%) | 14.0±0.1 | 14.0±0.1 | 14.0±0.0 |
| #matches: 407 | Sampson err. | 3.1±0.7 | 3.1±0.8 | 3.1±0.3 |
| | #samples | 13134±285 | 13267±547 | 18388±8 |
| 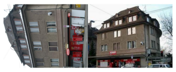 | #fitting | 1643±51 | 1680±62 | 2283±32 |
| | #verification | 1643±51 | 1680±62 | 36±5 |
| | runtime [sec] | 0.021±0.002 | 0.015±0.001 | 0.020±0.003 |
| **object 69 views 1 3** | inlier rate (%) | 33.2±0.0 | 33.2±0.0 | 33.2±0.0 |
| #matches: 316 | Sampson err. | 5.1±0.0 | 5.1±0.0 | 5.1±0.3 |
| | #samples | 396±4 | 396±9 | 554±133 |
| 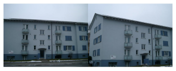 | #fitting | 74±10 | 81±5 | 111±18 |
| | #verification | 74±10 | 81±5 | 4±2 |
| | runtime [sec] | 0.002±0.000 | 0.002±0.000 | 0.005±0.000 |
| **object 167 views 3 5** | inlier rate (%) | 85.8±0.0 | 85.8±0.0 | 85.8±0.0 |
| #matches: 949 | Sampson err. | 2.4±0.3 | 2.4±0.2 | 2.4±0.0 |
| | #samples | 6±0 | 7±1 | 9±1 |
| 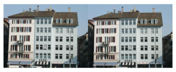 | #fitting | 5±1 | 5±1 | 8±1 |
| | #verification | 5±1 | 5±1 | 4±1 |
| | runtime [sec] | 0.013±0.004 | 0.012±0.001 | 0.015±0.001 |

Table 12. **Homography estimation on Zurich Buildings [4].**

## References


[1] S. Choi, Q.-Y. Zhou, and V. Koltun. Robust reconstruction of indoor scenes. In *IEEE Conference on Computer Vision and Pattern Recognition (CVPR)*, 2015. 2

[2] A. Kendall, M. Grimes, and R. Cipolla. Posenet: A convolutional network for real-time 6-dof camera relocalization. In *Computer Vision (ICCV), 2015 IEEE International Conference on*, pages 2938–2946. IEEE, 2015. 2, 3, 4, 9, 10

[3] K. Mikolajczyk and C. Schmid. Scale & affine invariant interest point detectors. *International journal of computer vision*, 60(1):63–86, 2004. 1, 2, 3, 4, 11

[4] H. Shao, T. Svoboda, and L. Van Gool. Zubud - zurich buildings database for image based recognition. *Computer Vision Lab, Swiss Federal Institute of Technology, Switzerland, Tech. Rep*, 260:20, 2003. 2, 3, 4, 12
